# Supplementary material for: End-to-End Video Object Detection with Spatial-Temporal Transformers
Source: arXiv:2105.10920 source file (2021-05-23)
Supplement: Supplementary file 1 [file 6appendix.tex]

\section{Appendix}
